# Supplementary material for: Medical Bill Shock and Imperfect Moral Hazard
Source: arXiv:2211.01116 source file (2024-03-04)
Supplement: Supplementary file 1 [file Appendix_LowValueServices.pdf]

| Category | Service | CPT Codes / Therapeutic Classes | Additional restrictions (age/sex restrictions, diagnosis or procedure codes) |
|---|---|---|---|
| All Pediatric | Vitamin D Screening | 82306,82652 | Age < 18 |
| All Pediatric | Cervical Cancer Screening | 87620,87621,87622, 87623, 87624, 87625, 88141, 88142, 88143, 88147, 88148, 88150, 88152, 88153, 88154, 88155, 88164, 88165,88166, 88167, 88174, 88175, G0123, G0124, G0141, G0143, G0144, G0145, G0147, G0148, P3000, P3001, Q0091 | Age < 18, age >= 14, female |
| All Pediatric | Head imaging for headache | 70450,70460,70470,70551,70552,70553 | Age < 18,<br>Diagnosis codes:<br>3390, 3391, 3460, 3461, 3462, 3464, 3465, 3467, 3468, 3469, 7840, 3393,<br>G440, G441, G442, G444, G430, G431, G435, G437, G438, G439, 30781,33983, 33984, 33985, R51, R510, R519, G4483, G4484, G4485 |
| All Pediatric | Antibiotics for upper respiratory infections | Antibiotics (multiple classes) | Diagnosis codes:<br>460,465, J00, J06, H65, H60, H61, H62, 3810, 3814 |
| All Pediatric | Antibiotics for bronchiolitis | Antibiotics (multiple classes) | Diagnosis codes: 46611,46619, J210, J218 |
| All Pediatric | Cough or cold medicine | Antitussives, Expectorants, Mucolytics, Cough/Cold Combinations | Age < 6 |
| | | | |
| Adult Drugs | Opioids to treat migraines | Opiate Agonists, Opiate Part Agonists, Opiate Antagonists | Diagnosis codes:<br>346**, G43** |
| | | | |
| Adult Imaging | Head imaging for headache | 70450,70460,70470,70551,70552,70553 | Diagnosis codes:<br>3390, 3391, 3460, 3461, 3462, 3464, 3465, 3467, 3468, 3469, 7840, 3393,<br>G440, G441, G442, G444, G430, G431, G435, G437, G438, G439, 30781,33983, 33984, 33985, R51, R510, R519, G4483, G4484, G4485 |
| Adult Imaging | Imaging for lower-back pain | 72010, 72020,72052, 72100, 72110, 72114,72120, 72200, 72202, 72220, 72131, 72132,<br>72133, 72141, 72142, 72146, 72147, 72148,72149, 72156, 72157, 72158 | Diagnosis codes:<br>7213, 7226, 7242, 7243, 7244,7245, 7246,7385, 7393,7394, 8460, 8461, 8462, 8463, 8468, 8469, 8472, M432, M512, M513, M518, M533, M545, M541, M543, M998, 72190, 72210, 72252, 72293, 72402,72470, 72471, 72479, M47817, M532X7, M9903, M9904,<br>S338XXA, S336XXA, S339XXA, S335XXA, M47819, M4647, M4806, M532X8 |

| Category | Service | CPT Codes / Therapeutic Classes | Additional restrictions (age/sex restrictions, diagnosis or procedure codes) |
|---|---|---|---|
| Adult Imaging | Screening for carotid artery disease | 36222, 36223, 36224, 70498, 70547, 70548,70549, 93880, 93882, 3100F | Diagnosis codes: 430, 431, 434,436,781, I63, I66, R25, R26, R27, R29, R47, G45, H34, R55, R20, 4350, 4351, 4353, 4358, 359,3623, 7802, 7820, I609, I619, 43301, 43311, 43321, 43331,43381, 43391, 99702, V1254, 36284, 78451, 78452, 78459, I6789, I67848, I97811, I97821, Z8673, H3582 |
| Adult Imaging | Cardiac imaging | 0144T, 0145T, 0146T, 0147T, 0148T, 0149T, 0150T, 75552, 75553, 75554, 75555, 75556, 75557, 75558, 75559, 75561, 75562, 75565, 75571, 75572, 75573, 75574, 78451, 78452, 78453, 78454, 78460, 78461, 78464, 78465, 78478, 78480, 78459, 78481, 78483, 78491, 78492, 78494, 78496, 78499 | |
| | | | |
| Adult Screening | Vitamin D Screening | 82306,82652 | |
| Adult Screening | Cardiac testing for low-risk patients | 93015, 93016, 93017, 93018, 93350, 93351,78451, 78452, 78453, 78454, 78460, 78461,78464, 78465, 78472, 78473, 78481, 78483,78491, 78492, 93303, 93304, 93306, 93307, 93308, 93312,93315, 93318, 3120F, 93000, 93005, 93010, G0366, G0367, G0368, G0403, G0404, G0405 | |
| Adult Screening | Pre-operative testing before low-risk surgery | 71010, 71015, 71020, 71021, 71022, 71023, 71030, 71034, 71035, 93303, 93304, 93306, 93307, 93308, 93312, 93315, 93318, 94010, 78451, 78452, 78453, 78454, 78460, 78461, 78464, 78465, 78472, 78473, 78481, 78483, 78491, 78492, 93015, 93016, 93017, 93018, 93350, 93351 | Procedure codes for surgery: 19120, 19125, 47562, 47563, 49560, 58558 |
| | | | |
| Adult Surgery | Arthroscopic surgery for knee osteoarthritis | 29877, 29879, G0289 | Diagnosis codes: 8360, 8361, 8362, 7170, S832, 71741, M23202, M23205 |

*Table Notes:* Pediatric low-value services are defined based on Chua et al. (2016). Adult low-value services are based on definitions given in Bhatia et al. (2015), Chandra et al. (2021), and Colla et al. (2014).
